# Supplementary material for: Countering Autonomous Cyber Threats
Source: arXiv:2410.18312 source file (2024-10-23)
Supplement: Supplementary file 1 [file appendix2.tex]

%!TEX root = ../thesis.tex
% ******************************* Thesis Appendix B ********************************

\chapter{Other stuff.}
